# Supplementary material for: Predicting scaling properties from a single fluid configuration
Source: arXiv:2105.12258 source file (2021-05-25)
Supplement: Supplementary file 1 [file Single_Supp_v5.pdf]

# Supplemental material - Predicting scaling properties from a single configuration

Thomas B. Schrøder*

*Glass and Time, IMFUFA, Department of Science and Environment,*

*Roskilde University, P.O. Box 260, DK-4000 Roskilde, Denmark*

(Dated: May 25, 2021)

* tbs@ruc.dk

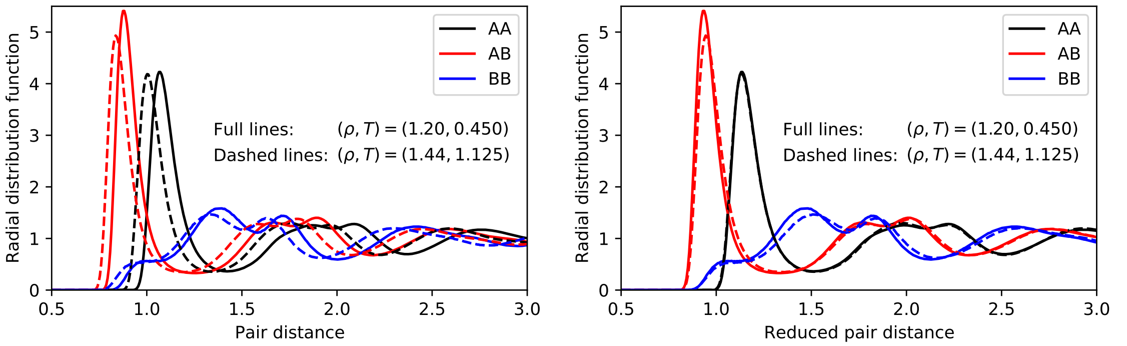


FIG. 1. Radial distribution function for the two state points $(\rho_1, T_1) = (1.20, 0.45)$ (full lines) and $(\rho_2, T_2) = (1.44, 1.125)$ (dashed lines). Left panel: MD units. Right panel: Reduced units. In the reduced units, the radial distribution functions are very similar, in particular for the AA-interaction, which is the majority.

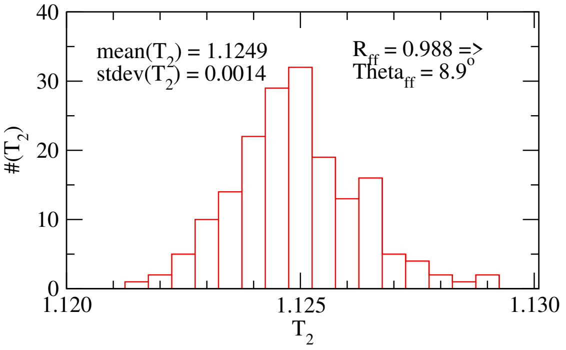


FIG. 2. Distribution of $T_2$ values predicted by 178 independent configurations at the reference state point $(\rho_1, T_1) = (1.20, 0.45)$, scaling to $\rho_2 = 1.44$.

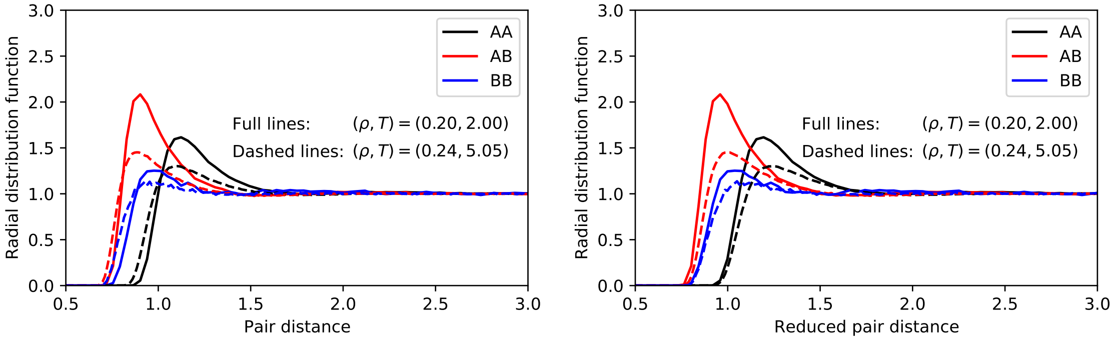


FIG. 3. Radial distribution function for the two state points $(\rho_1, T_1) = (0.20, 2.00)$ (full lines) and $(\rho_2, T_2) = (0.24, 5.05)$ (dashed lines), where $T_2 = 5.05$ is the result of applying Eq.(2) of the main text to a configuration at the low density reference state point $(\rho_1, T_1) = (0.20, 2.00)$ . Left panel: MD units. Right panel: Reduced units. The structure is far from invariant (compare Fig. 1 above), reflecting that the scaling properties found at high densities does not apply here.

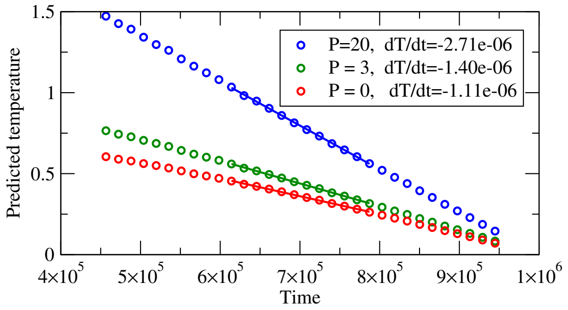


FIG. 4. Estimating 'isomorphic' cooling rate from P=10 cooling curve, see Fig. 5. of main text.
